# Supplementary material for: Efficient Constrained Dynamics Algorithms based on an Equivalent LQR Formulation using Gauss' Principle of Least Constraint
Source: arXiv:2310.00688 source file (2023-10-01)
Supplement: Supplementary file 1 [file appendixA.tex]

We derive the equivalent joint torques $\boldsymbol{\tau}^c$ to show the inconsistency of Vereshchagin's suggestion in \cref{eq:Vere_tsid} with \cref{eq:Jac_tsid}. We use a kinematic chain with only an end-effector constraint in this derivation. Let $\mathbf{f}_i^c$ be the reaction force propagated to link $i$ due to $\boldsymbol{\tau}^c$ applied on $i$-th link's descendants. $\boldsymbol{\tau}^c_i$ and $\mathbf{f}_i^c$ acting on any link $i$ must cause the same $\mathbf{\ddot{q}}_i^*$ as the constraint force $(K_i^{AT}\boldsymbol{\lambda}^*)$, which for all joints requires,

\begin{equation} \label{eq:eq_torque_con}
\boldsymbol{\tau}_i^c + S_i^Tf_i^c = -S_i^T(K_i^{AT}\boldsymbol{\lambda}^*).
\end{equation}

For the end-effector joint, $\mathbf{f}_n^c = 0$ as there are no descendant links and joints to cause a reaction force. Therefore, 
\begin{equation} \label{eq:tau_n}
\boldsymbol{\tau}_n^c = -S_n^T(K_n^{AT}\boldsymbol{\lambda}^*),
\end{equation}

and reaction force on the $n-1$-th link because of $\boldsymbol{\tau}_n^c$ is 
\begin{equation} \label{eq:reaction_force}
\mathbf{f}_{n-1}^c = -H_n^AS_n(D_n)^{-1}\boldsymbol{\tau}_n^c.
\end{equation}

The equivalent torque condition in \cref{eq:eq_torque_con} for the $n-1$-th joint after substituting \cref{eq:reaction_force} is

\begin{subequations}
\begin{align}
\boldsymbol{\tau}_{n-1}^c + &S_{n-1}^T\mathbf{f}_{n-1}^c  = -S_{n-1}^T(K_{n-1}^{AT}\boldsymbol{\lambda}^*) \\
& = -S_{n-1}^T(P_nK_{n}^{AT}\boldsymbol{\lambda}^*) \\ 
& = -S_{n-1}^T( \mathbf{1}_{6 \times 6} - H_n^AS_n(D_n)^{-1}S_n^T)K_{n}^{AT}\boldsymbol{\lambda}^* \\
& = -S_{n-1}^T(K_{n}^{AT}\boldsymbol{\lambda}^* + H_n^AS_n(D_n)^{-1}\boldsymbol{\tau}_n^c) \\
& = -S_{n-1}^T(K_{n}^{AT}\boldsymbol{\lambda}^* - \mathbf{f}_{n-1}^c).
\end{align}
\end{subequations}

Subtracting $S_{n-1}^T\mathbf{f}_{n-1}^c$ to both sides of the equation above gives

\begin{equation}
\boldsymbol{\tau}_{n-1}^c = -S_{n-1}^TK_{n}^{AT}\boldsymbol{\lambda}^*, 
\end{equation}

which differs from Vereshchagin suggestion in \cref{eq:Vere_tsid}. Continuing this process backwards in the chain, the reaction force at the $n-2$-th due to the additional joint torques is

\begin{equation}
\mathbf{f}_{n-2}^c = -H_{n-1}^AS_{n-1}(D_{n-1})^{-1}\boldsymbol{\tau}_{n-1}^c + P_{n-1}\mathbf{f}_{n-1}^c.
\end{equation}

Repeating the equivalent torque condition \cref{eq:eq_torque_con} for $n-2$-th joint, with some re-arrangement of terms we get

\begin{subequations} \label{eq:tsid_der}
\begin{align} 
\boldsymbol{\tau}_{n-2}^c &+ S_{n-2}^T(\mathbf{f}_{n-2}^c) \\
&= -S_{n-2}^T(K_{n-2}^{AT}\boldsymbol{\lambda}^*) \\
& = -S_{n-2}^T(P_{n-1}K_{n-1}^{AT}\boldsymbol{\lambda}^*) \\
& = -S_{n-2}^T(P_{n-1}(K_{n}^{AT}\boldsymbol{\lambda}^* - \mathbf{f}_{n-1}^c)) \\
& = -S_{n-2}^T( P_{n-1}K_{n}^{AT}\boldsymbol{\lambda}^* - P_{n-1}\mathbf{f}_{n-1}^c) \\
& = -S_{n-2}^T(K_{n}^{AT}\boldsymbol{\lambda}^* + H_{n-1}^AS_{n-1}(D_{n-1})^{-1}\boldsymbol{\tau}_{n-1}^c - \nonumber \\ & \qquad P_{n-1}\mathbf{f}_{n-1}^c) \\
&= -S_{n-2}^T(K_{n}^{AT}\boldsymbol{\lambda}^* - \mathbf{f}_{n-2}^c).
\end{align}
\end{subequations}

Substracting $S_{n-2}^T(\mathbf{f}_{n-2}^c)$ from both sides of the equation above gives 
\begin{equation}
\boldsymbol{\tau}_{n-2}^c = -S_{n-2}^T(K_{n}^{AT}\boldsymbol{\lambda}^*).
\end{equation}	

The same steps in \cref{eq:tsid_der} can be repeated for all the joints in the chain to get the general equation

\begin{equation} \label{eq:Correct_tsid}
\boldsymbol{\tau}_{i}^c = -S_{i}^T(K_{n}^{AT}\boldsymbol{\lambda}^*).
\end{equation}

 %such that generalized forces that need to by supplied by joint motors to realize the desired acceleration constraints is $\boldsymbol{\tau}_i +  \boldsymbol{\tau}_{\mathrm{add},i}$. However, we report that following this suggestions does not lead to the correct computation of task-space hybrid dynamics. This is because the equivalent generalized forces for a constraint wrench $K_i^T\mathbf{\boldsymbol{\lambda}^*_i}$ acting on the $i$-th link obeys the following relationship \cite[Section 6.1.2]{murray2017mathematical}, \cite[eq. 8.31]{featherstone2014rigid}

%\begin{equation} \label{eq:Correct_tid}
%\boldsymbol{\boldsymbol{\tau}}_\mathrm{add} = \sum_{i = 1}^n J_i^T(K_i^T\boldsymbol{\boldsymbol{\lambda}^*}) 
%\end{equation}

Since $S_i$ is precisely the $i$-th column of the geometric Jacobian $J_n$, the above formula can be re-stated as the familiar equation that maps spatial forces to joint torques
\begin{equation}
\boldsymbol{\tau}^c = J_n^T(-K_{n}^{AT}\boldsymbol{\lambda}^*) = J^T\boldsymbol{\lambda}^*,
\end{equation}

with the last equality due to our assumption that only the end-effector is constrainted. Vereshchagin's suggestion in \cref{eq:Vere_tsid} gives inconsistent inverse dynamics torques essentially because it does not properly account for the reaction forces that must be propagated backwards due the equivalent joint torques $\boldsymbol{\tau}^c$.
